# Supplementary material for: Stabilizing language models under continual learning via condition-anchored distillation
Source: arXiv:2610.06940 source file (2026-10-03)
Supplement: Supplementary file 1 [file cagd_qualitative_additional.tex]

\begin{table}[H]
\centering
\caption{GSM8K outputs after the \emph{GSM8K $\rightarrow$ summarization $\rightarrow$
creative-writing} stream.  To expose the mixed aggregate result rather than
select only gains, rows are the lowest test indices in three strata among
questions answered correctly when learned: both methods correct,
Sequential-only correct, and \CAGD{}-only correct.  The left column
instantiates the input and target templates; the original rationale is elided
for space. Model: SMDM-219M}
\label{tab:smdm-gsm8k-examples}
\scriptsize
\setlength{\tabcolsep}{3pt}
\renewcommand{\arraystretch}{1.08}
\begin{tabular}{@{}p{0.22\textwidth}p{0.36\textwidth}p{0.36\textwidth}@{}}
\toprule
\tablehead{Input and target} & \tablehead{Sequential final output} & \tablehead{\CAGD{} final output}\\
\midrule
\texttt{Question:} A water tank is filled with 120 liters of water. Celine used 90 liters of
water from the tank to water her small garden. She was then able to collect
rainwater that is twice as much as what was left. How many liters of water are
in the tank now?\par
\texttt{Answer:}\par\smallskip
\textbf{Target template}\par
\texttt{<original rationale>}\par
\texttt{\#\#\#\# 90}
& \emph{Parsed: 90 (correct).} The tank is full of water. The water is very
hot, and she used 90 liters of water. The water is not very hot, and she is
not able to soak the water. Her rainwater is twice as full, and she is now
able to\ldots
& \emph{Parsed: 90 (correct).} The water tank is filled with 120 liters of
water. The water is 90 liters of water. The water is 90 liters of water. The
water is 90 liters of water. The water is 90 liters of water. The water is 90
liters of water.\\
\addlinespace
\texttt{Question:} Lindsay is doing the laundry, and thinks she has missed some socks. There are
50 socks that need washing. If she washes 10 pairs of socks and 15 loose
socks, how many socks has Lindsay missed?\par
\texttt{Answer:}\par\smallskip
\textbf{Target template}\par
\texttt{<original rationale>}\par
\texttt{\#\#\#\# 15}
& \emph{Parsed: 15 (correct).} Lindsay has missed 50 socks. Lindsay washed 10
pairs of socks and 15 loose socks. Lindsay washed 10 pairs of socks and 15
loose socks. Lindsay has missed Lindsay's sock, which is also full of loose
socks. Lindsay has missed Lindsay's sock, which is also\ldots
& \underline{\emph{Parsed: 10 (incorrect).}} Lindsay washes 10 pairs of socks and 15
loose socks. So she washes 10 pairs of socks and 15 loose socks. So she
washes 10 pairs of socks and 15 loose socks. So she washes 10 pairs of socks
and 15 loose socks. So she\ldots\\
\addlinespace
\texttt{Question:} Jared is trying to increase his typing speed. He starts with 47 words per
minute (WPM). After some lessons the next time he tests his typing speed it
has increased to 52 WPM. If he continues to increase his typing speed once
more by 5 words, what will be the average of the three measurements?\par
\texttt{Answer:}\par\smallskip
\textbf{Target template}\par
\texttt{<original rationale>}\par
\texttt{\#\#\#\# 52}
& \emph{Parsed: none (incorrect).} Jared is trying to increase his typing
speed. The first way is to increase his typing speed. The second way is to
increase his typing speed. The third way is to increase his typing speed. The
fourth way is to increase his typing speed. The\ldots
& \textbf{\emph{Parsed: 52 (correct).}} First he will increase his typing speed by 47
words per minute. Then he will increase his typing speed by 52 words per
minute. Then he will increase his typing speed by 52 words per minute.
Finally he will increase his typing speed by 52\ldots\\
\bottomrule
\end{tabular}
\end{table}

\begin{table}[H]
\centering
\caption{Final held-out \emph{summarization} outputs
after the \emph{closed QA $\rightarrow$ summarization $\rightarrow$
creative-writing} stream. The three IDs were fixed from their inputs before
generation. Full prompts, references, and unedited outputs are retained in
the qualitative artifacts.  The left column shows the exact input template
and dataset target. Model: Qwen3-0.6B}
\label{tab:qwen-summarization-examples}
\scriptsize
\setlength{\tabcolsep}{3pt}
\renewcommand{\arraystretch}{1.08}
\begin{tabular}{@{}p{0.28\textwidth}p{0.33\textwidth}p{0.33\textwidth}@{}}
\toprule
\tablehead{Input and target} & \tablehead{Sequential final output} & \tablehead{\CAGD{} final output}\\
\midrule
\texttt{Instruction:} What is dhollywood?\par
\texttt{Context:} Gujarati cinema, also known
as Dhollywood, is the Gujarati language film industry. It is one of the major
regional and vernacular film industries of the cinema of India, having
produced more than one thousand films since its inception.\par
\texttt{Response:}\par\smallskip
\textbf{Target}\par
Dhollywood is a nickname for movies made by Gujarati cinema in India.
& Dhollywood is a fictional story. Dhollywood is a fictional story.
Dhollywood is a fictional story. Dhollywood is a fictional story. Dhollywood
is a fictional story. Dhollywood is a fictional story. Dhollywood is a
fictional story. Dhollywood is a fictional story.
& \textbf{Dhollywood is a nickname for Gujarati cinema.}\\
\addlinespace
\texttt{Instruction:} Please give me the list of airports that are owned by
Australia Pacific Airports Corporation.\par
\texttt{Context:} Australia Pacific Airports
Corporation Limited (APAC) is an unlisted company and owner of two Australian
airports: Melbourne Airport and Launceston Airport. Each airport is operated
by an airport lessee company, in which APAC has a controlling interest:
Australia Pacific Airports (Melbourne) Pty Ltd and Australia Pacific Airports
(Launceston) Pty Ltd respectively.\par
\texttt{Response:}\par\smallskip
\textbf{Target}\par
Australia Pacific Airports
Corporation Limited owns two airports in Australia called Launceston Airport
and Melbourne Airport.
& The purpose of this query is to find out the airports that are owned by the
corporation. The cities of interest are: 38 and 39.
& \textbf{The company has a controlling interest in: 1. Melbourne Airport and 2.
Launceston Airport.}\\
\addlinespace
\texttt{Instruction:} How many people attended the Summer Breeze Open Air?\par
\texttt{Context:} Summer Breeze Open Air is an annual German heavy metal music
festival. It was first held in 1997. The festival had been held in
Abtsgm\"und until 2006 when it was moved to its new location of
Dinkelsb\"uhl, Bavaria. The festival draws around 40,000 attendees annually.
\par\texttt{Response:}\par\smallskip
\textbf{Target}\par
The German heavy metal music festival Summer Breeze Open Air drew 40,000
attendees annually.
& Summer Breeze has an effect on the number of people who attended the
festival. While effect is attribute of effect, effect is attribute of effect.
& Summer Breeze was held in Dinkelsb\"uhl, Bavaria.\\
\bottomrule
\end{tabular}
\end{table}

\begin{table}[H]
\centering
\caption{Final held-out \emph{creative-writing} outputs
from the same model pair and natural-task stream as
\cref{tab:qwen-summarization-examples}.  The task is open-ended, so the table
shows instruction following rather than treating the dataset response as a
unique correct target.  The left column shows the exact input template and
dataset target. Model: Qwen3-0.6B.}
\label{tab:qwen-writing-examples}
\scriptsize
\setlength{\tabcolsep}{3pt}
\renewcommand{\arraystretch}{1.08}
\begin{tabular}{@{}p{0.30\textwidth}p{0.32\textwidth}p{0.32\textwidth}@{}}
\toprule
\tablehead{Input and target} & \tablehead{Sequential final output} & \tablehead{\CAGD{} final output}\\
\midrule
\texttt{Instruction:} Write a dialogue between two hikers, John and Jane, who are lost in the woods
and can't decide what to do. End the argument with Jane winning and them
deciding to turn around and retrace their steps.\par
\texttt{Response:}\par\smallskip
\textbf{Target}\par
John: I think we're lost, this trail doesn't look familiar\newline
Jane: I think you're right. We must have taken a wrong turn at the fork a mile
back. Let's turn around and trace our steps back\newline
John: No, I think we should just keep going forward. We are still on a path,
so we should just go and see if we can find our way back to a path we
know\newline
Jane: I'm worried its going to get dark, and we'll just be going further into
the woods. We should turn around and repeat our steps\newline
John: Okay, you're right. Let's go back to where we first got lost and take the
other side of the fork.
& Before I lost track of time and energy, John and Jane explained their
reasons for being lost and the conversation went through. They agreed upon a
way to proceed and Jane suggested a way to find the way home.
& The last exchange is a conditional. The conditional is conditional on
Jane's last word.\\
\addlinespace
\texttt{Instruction:} Write a poem about George Washington.\par
\texttt{Response:}\par\smallskip
\textbf{Target}\par
George Washington was a British man\newline
The British had laws he couldn't understand\newline
Washington and his friends put together a plan\newline
That the people would resist and America could stand
& The last man on earth, he still stands, he still sees what we do in here,
he still sees what I've done in here, I'll keep on going, I'll keep on going,
I'll keep on going, I'll keep on going, I'll keep on going, I'll\ldots
& The last man on earth, he was the father of our nation, the origin of our
government, the inspiration of our nation. I am amazed by the greatness of
our nation. I hope to visit the country one day and witness the greatness of
our\ldots\\
\addlinespace
\texttt{Instruction:} Write me a thank you note for my high-school teacher\par
\texttt{Response:}\par\smallskip
\textbf{Target}\par
Thank you for being a supportive teacher and encouraging me to keep learning.
I will always remember your encouragement as I move forward in my studies.
& Hi, I hope you have been in good health! I'm so excited to inform you that
I'm almost finished my first year in my major field of interest. I'm so
excited to inform you that I'm almost finished my first year in my major
field\ldots
& The teacher's name, Nick, is a huge part of this note. He's a huge part of
all of us, from when we were kids to today, he's been a huge part in our
education and in our growth. I hope to continue to be in\ldots\\
\bottomrule
\end{tabular}
\end{table}
